# Supplementary material for: Scout: Rapid Exploration of Interface Layout Alternatives through High-Level Design Constraints
Source: arXiv:2001.05424 source file (2020-01-15)
Supplement: Supplementary file 1 [file 9_supplementary_materials.tex]

\clearpage
\section{Supplementary Materials}
\subsection{Spatial Diversity Score}
Here we include the formalized equation for the spatial diversity score we used for our evaluation. We compute a spatial diversity score for a pair of designs by computing for each pair of matching elements (1) the difference in position (i.e., x,y - diagonal), (2) the difference in area (i.e., $width * height$), and (3) relative distance change between any pair of elements. 

First, the \emph{position difference score} $s_\mathit{dist}$ computes the average position change between the centers for each matching element in the two layouts. Given two layouts $L$ and $L'$ with elements $L=\{e_1,\dots,e_n\}$ and $L'=\{e'_1,\dots,e'_n\}$, Scout calculates $s_\mathit{dist}$ as follows:
    $$s_\mathit{dist}(L, L')=\frac{1}{n}\cdot\sum_{i=1}^n\sqrt{(e.x-e'.x)^2 + (e.y-e'.y)^2}$$
% Discuss normalization later 
% where the scoring function measures the normalized absolute distance between the centers of the the two element.
    %The normalization constant $\sqrt{W^2 + H^2}$ is the diagonal length of the canvas (with width $W$ and height $H$), which ensures that the score to be in range $[0,1)$.
Second, we compute a \emph{size change score} $s_\mathit{size}$ to measure the average change in size for each matching pair of elements in the two layouts. Given two layouts $L=\{e_1,\dots,e_n\}$ and $L'=\{e'_1,\dots,e'_n\}$, Scout calculates $s_\mathit{size}$ as follows:
    $$s_\mathit{size}(L, L')=\frac{1}{n}\cdot\sum_{i=1}^n |e_i.width \cdot e_i.height - e_i'.width\cdot e_i'.height|$$
    % where $e.h$ and $e.w$ refers to heights and width of each elements.
    %and the normalizing constant $W\cdot H$ is the size of the canvas.
    
Third, we compute a \emph{relational distance score} score to measure how much each element moved in relation to all other elements in the layout.  Given two layouts  $L=\{e_1,\dots,e_n\}$ and $L'=\{e'_1,\dots,e'_n\}$, we calculate the relational distance score $s_\mathit{rel}$ as follows:
    $$s_\mathit{rel}(L, L')=\frac{2}{n(n-1)}\cdot\sum_{1\le i< j\le n}|\mathit{dist}(e_i,e_j)-\mathit{dist}(e_i',e_j')|$$
    where $\mathit{dist}(e_i,e_j)=\sqrt{(e_i.x-e_j.x)^2 + (e_i.y-e_j.y)^2}$ calculates the distance between centers of the two elements.  
    
Finally, we compute a spatial diversity score $s_\mathit{diversity}$ as the weighted sum of the three metrics $s_\mathit{dist}, s_\mathit{size}, s_\mathit{rel}$:
$$s_\mathit{diversity}=w_\mathit{dist}\cdot s_\mathit{dist} + w_\mathit{size}\cdot s_\mathit{size} + w_\mathit{rel}\cdot s_\mathit{rel}$$

To ensure each metric is weighted equally, we normalize the metrics into the range $[0,1]$. Given the entire set of layouts designers created in our evaluation $\{L_1,\dots L_n\}$, we compute the weights
$w_\mathit{dist}=\frac{1}{\mathit{max\_dist\_change}}$, $w_\mathit{size}=\frac{1}{\mathit{max\_size\_change}}$, $w_\mathit{rel}=\frac{1}{\mathit{max\_rel\_dist\_change}}$. 
where each weight ($w_\mathit{dist}$, $w_\mathit{size}$, $w_\mathit{rel}$ is the maximum distance, size, and relational distance change for any pair of elements in the evaluation set $L_i,L_j$, respectively.

% -- TODO: Decide if constraint equation needed. 
% Ordering 
% \begin{equation}
% \label{equation6}
%     \begin{multlined}
%         \phi_{baseline\_grid} := \forall_{i=1}^{E}e_{i}.x == e_{i}.y \bmod c.b\_grid == 0 \\
%         \shoveleft[3cm]{\&\: e_{i}.height \bmod c.b\_grid == 0} \\
%     \end{multlined}
% \end{equation}
% \vspace{-1em}
